# Supplementary material for: Precision benchmarks for solids: G0W0 calculations with different basis sets
Source: arXiv:2411.19701 ancillary file (2024-11-29)
Supplement: Supplementary file 1 [file Supplemental_Material.pdf]

# Precision benchmarks for solids: $G_0W_0$ calculations with different basis sets

Maryam Azizi,[1,2,*] Francisco A. Delesma,[3,4] Matteo Giantomassi,[1,2] Davis Zavickis,[5] Mikael Kuisma,[6] Kristian Thyghesen,[6] Dorothea Golze,[4] Alexander Buccheri,[7] Min-Ye Zhang,[8] Patrick Rinke,[3] Claudia Draxl,[7,2] Andris Gulans,[5] and Xavier Gonze[1,2]

[1] *Université Catholique de Louvain, Louvain-la-Neuve, Belgium*

[2] *European Theoretical Spectroscopic Facility (ETSF)*

[3] *Department of Applied Physics, Aalto University, FI-02150 Espoo, Finland*

[4] *Faculty for Chemistry and Food Chemistry, Technische Universität Dresden, 01062 Dresden, Germany*

[5] *University of Latvia, Riga, Latvia*

[6] *Danish Technical University, Lyngby, Denmark*

[7] *Humboldt-Universität zu Berlin, Berlin, Germany*[†]

[8] *The NOMAD Laboratory at the Fritz Haber Institute of the Max Planck Society, Berlin, Germany*

(Dated: November 29, 2024)

## I. REDUCED CARTESIAN COORDINATES FOR THE BENCHMARKED SYSTEMS

TABLE S1. Atomic positions in reduced coordinates for $ZrO_2$ structure

| x | y | z |
|---|---|---|
| 0.000 | 0.000 | 0.000 |
| 0.250 | 0.250 | 0.250 |
| 0.750 | 0.750 | 0.750 |

* maryam.azizi@uclouvain.be

† New address of A. Buccheri: Max Planck Institute for the Structure and Dynamics of Matter, Hamburg, Germany

TABLE S2. Atomic positions in reduced coordinates for $Zr_2Y_2O_7$

| **x** | **y** | **z** |
|---|---|---|
| 0.042915780 | 0.985388339 | 0.991757333 |
| 0.052825879 | 0.437198758 | 0.525285780 |
| 0.497849315 | 0.475347221 | 0.021504009 |
| 0.490855515 | 0.976347566 | 0.462963104 |
| 0.225142926 | 0.214346603 | 0.246291488 |
| 0.299171805 | 0.212877989 | 0.738681316 |
| 0.201778352 | 0.719375074 | 0.271586001 |
| 0.210239202 | 0.723023653 | 0.756618977 |
| 0.706459701 | 0.368427306 | 0.368842334 |
| 0.831742406 | 0.281842589 | 0.827464461 |
| 0.691019058 | 0.855824888 | 0.088167548 |

TABLE S3. Atomic positions in reduced coordinates for $MoWS_4$

| **x** | **y** | **z** |
|---|---|---|
| 0.000 | 0.000 | 1.25346149 |
| 2/3 | 1/3 | 1.37960867 |
| 2/3 | 1/3 | 1.12731281 |
| 0.000 | 0.000 | 1.87881941 |
| 0.000 | 0.000 | 1.62814874 |
| 2/3 | 1/3 | 1.75348588 |

TABLE S4. Atomic positions in reduced coordinates for silicon

| **x** | **y** | **z** |
|---|---|---|
| 0.000 | 0.000 | 0.000 |
| 0.250 | 0.250 | 0.250 |

TABLE S5. Atomic positions in reduced coordinates for $TiO_2$

| x | y | z |
|---|---|---|
| 0.000 | 0.000 | 0.000 |
| 0.500 | 0.500 | 0.500 |
| 0.303779258 | 0.303779258 | 0.000 |
| 0.696220742 | 0.696220742 | 0.000 |
| 0.803779258 | 0.196220742 | 0.500 |
| 0.196220742 | 0.803779258 | 0.500 |

TABLE S6. Atomic positions in reduced coordinates for ZnO

| x | y | z |
|---|---|---|
| 1/3 | 2/3 | 0.000 |
| 2/3 | 1/3 | 0.500 |
| 1/3 | 2/3 | 0.3821000000 |
| 2/3 | 1/3 | 0.8821000000 |

## II. FHI-AIMS BASIS SET CONVERGENCE

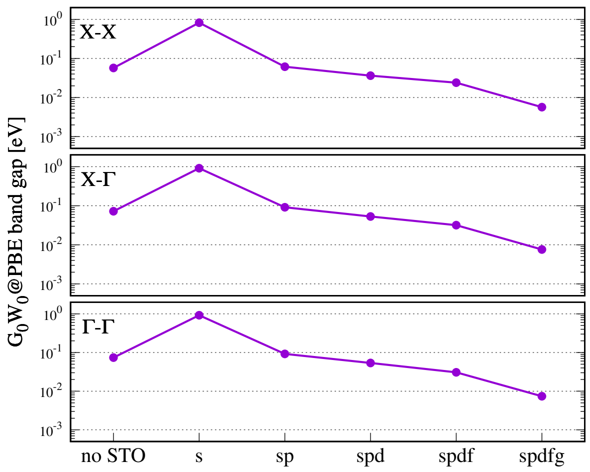


FIG. S1. Convergence of the $ZrO_2$ bandgap with respect to the increment of higher angular momentum in STO.

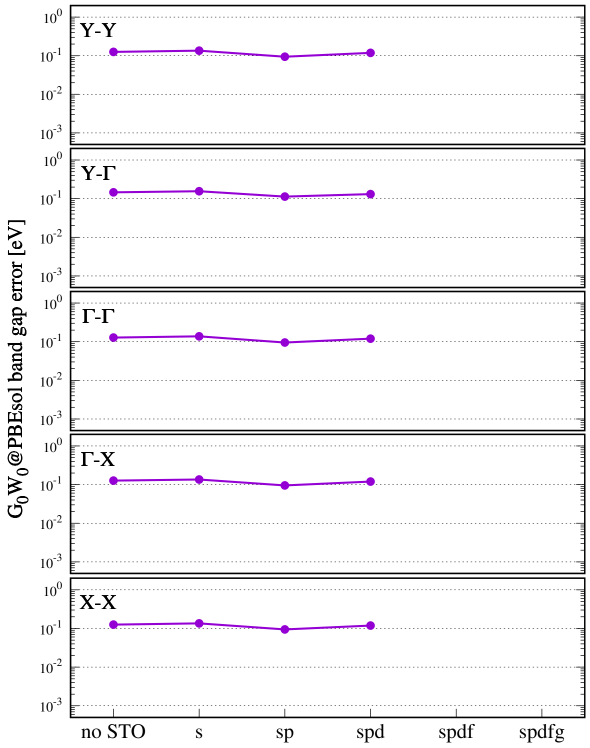


FIG. S2. Convergence of the $Zr_2Y_2O_7$ bandgap with respect to the increment of higher angular momentum in STO.

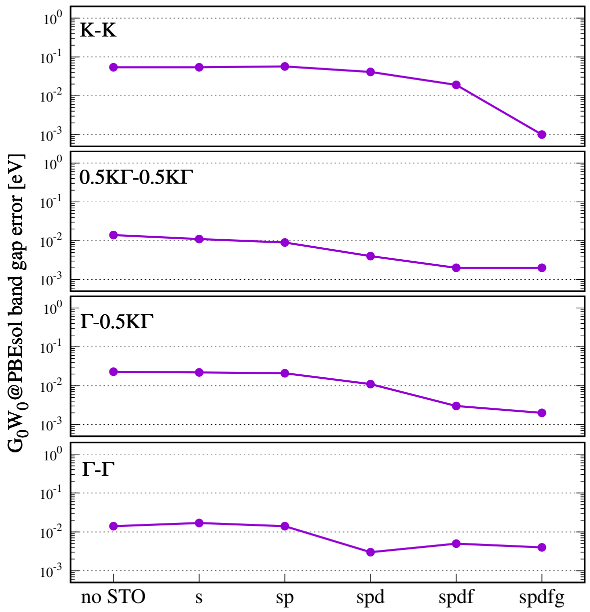


FIG. S3. Convergence of the $MoWS_2$ bandgap with respect to the increment of higher angular momentum in STO.

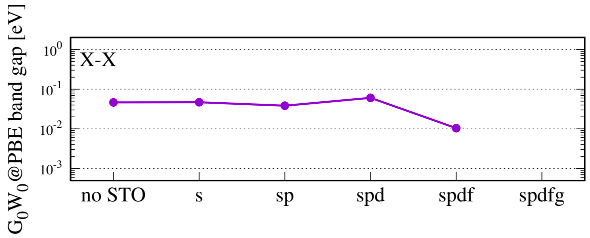


FIG. S4. Convergence of the $TiO_2$ bandgap with respect to the increment of higher angular momentum in STO.
